# Supplementary material for: Applying Machine Learning to Life Insurance: some knowledge sharing to master it
Source: arXiv:2209.02057 source file (2022-09-27)
Supplement: Supplementary file 1 [file algo_sourceAL.tex]

\subsection{Arbres, Bagging et Forêts Aléatoires}\label{sec:arbres:forets}

Les arbres de classification ont été introduits dans \cayNP{Quinlan} mais c'est surtout \cayNP{Breiman} qui a assuré la popularité de l'algorithme. On parle de modèle CART pour « {\em Classification And Regression Tree} ». 
L'idée est de diviser consécutivement (par une notion de branchement) les données d'entrée jusqu'à ce qu'un critère d'affectation (par rapport à la variable cible) soit atteint, selon une règle prédéfinie. 

L'intuition de la construction des arbres de classification est la suivante. L'entropie $H (\boldsymbol{x})$ est associée à la quantité de désordre dans les données $\boldsymbol{x}$ par rapport aux modalités prises par la variable de classification $y$, et chaque partition vise à réduire ce désordre. L'interprétation probabiliste est de créer les groupes les plus homogènes possible, en réduisant la variance par groupe (variance intra), ou de manière équivalente en créant deux groupes aussi différents que possible, en augmentant la variance entre les groupe (variance inter).
à chaque étape, nous choisissons la partition qui donne la plus forte réduction de désordre (ou de variance). L'arbre de décision complet se développe en répétant cette procédure sur tous les sous-groupes, où chaque étape $k$ aboutit à une nouvelle partition en 2 branches, qui subdivise notre ensemble de données en 2. Enfin, on décide quand mettre fin à cette constitution de nouvelles branches, en procédant à des affectations finales (n\oe{}uds dits foliaires). Il existe plusieurs options pour mettre fin à cette croissance. L'une est de construire un arbre jusqu'à ce que toutes les feuilles soient pures, c'est à dire composées d'une seule observation. Une autre option est de définir une règle d'arrêt liée à la taille, ou à la décomposition, des feuilles. Les exemples de règles d'arrêt peuvent être d'une taille minimale (au moins 5 éléments par feuille), ou une entropie minimale. On parlera alors d'élagage de l'arbre: \revision{on laisse l'arbre grossir, puis on coupe certaines branches {\em a posteriori} (ce qui est différent de l'introduction d'un critère d'arrêt {\em a priori} au processus de croissance de l'arbre - par exemple en imposant une taille minimale aux feuilles, ou d'autres critères discutés dans \cayNP{Breiman}).}

à un n\oe{}ud donné, constitué de $n_0$ observations $(\boldsymbol{x}_i,y_i)$ avec $i\in\mathcal{I}_0$, on va couper en deux branches (une à gauche et une à droite), partitionnant ainsi $\mathcal{I}_0$ en $\mathcal{I}_{\text{g}}$ et $\mathcal{I}_{\text{d}}$. Soit $I$ le critère d'intérêt, comme l'entropie du n\oe{}ud (ou plutôt du n\oe{}ud vu en tant que feuille):
$$
I(\boldsymbol{y}_0)=-n_0 p_0\log p_0 \text{\quad où \quad}p_0=\frac{1}{n_0}\sum_{i\in\mathcal{I}_0}y_i, 
$$
ou la variance du n\oe{}ud:
$$
I(\boldsymbol{y}_0)=n_0 p_0(1- p_0) \text{\quad où \quad}p_0=\frac{1}{n_0}\sum_{i\in\mathcal{I}_0}y_i, 
$$
ce dernier étant également l'indice \revision{d'impureté} de Gini. 

\begin{figure}[h]
\centering
\caption{Schéma d'illustration d'un arbre de décision permettant de prédire le taux de survie d'un individu du Titanic.}
\vspace{0.5cm}
%\includegraphics[width=.9\textwidth,height=.45\textheight]{rpartTitanic}
\begin{tikzpicture}[sibling distance=10em,
  good/.style = {shape=rectangle, rounded corners,
    draw, align=center, top color=white, bottom color=green!20},
  bad/.style = {shape=rectangle, rounded corners,
    draw, align=center, top color=white, bottom color=red!20}
]]
  \node(A) {\bf homme?}
    child { node(B1) {\bf âge$\,>\,$9.5? } 
	child { node[bad](C1) {décès \\ {\footnotesize 0.17 61\%}} }
	child { node(C2) {\bf {\sffamily sibsp}$\,>\,$2.5?} 
		child { node[bad](D1) {décès \\ {\footnotesize 0.05 2\%}}} 
		child { node[good](D2) {survie \\ {\footnotesize 0.89 2\%}}} 
}
}
    child { node[good](B2) {survived\\ {\footnotesize 0.73 36\%}} };
  % Labels
  \begin{scope}[nodes = {draw = none}]
    \path (A)     -- (B1) node [near start, left]  {\footnotesize \em yes};
    \path (A)     -- (B2) node [near start, right] {\footnotesize \em non};
    \path (B1) -- (C1) node [near start, left] {\footnotesize \em oui};
    \path (B1) -- (C2) node [near start, right] {\footnotesize \em non};
    \path (C2) -- (D1) node [near start, left] {\footnotesize \em oui};
    \path (C2) -- (D2) node [near start, right] {\footnotesize \em non};
 \end{scope}
\end{tikzpicture}
\label{cart_titanic}
\end{figure}

On partitionnera entre la branche gauche et la branche droite si le gain $I(\boldsymbol{y}_0)-\big[I(\boldsymbol{y}_{\text{g}})+I(\boldsymbol{y}_{\text{d}})\big]$ 
est suffisamment important. Lors de la construction des arbres, on va chercher la partition qui donne le gain le plus important possible. Ce problème combinatoire étant complexe, le critère suggéré par \cayNP{Breiman} est de considérer un découpage suivant une des variables, avec $\mathcal{I}_{\text{g}}=\lbrace i\in\mathcal{I}_0:x_{k,i}<s\rbrace$ et $\mathcal{I}_{\text{d}}=\lbrace i\in\mathcal{I}_0:x_{k,i}>s\rbrace$, pour une variable $k$ et un seuil $s$ (si la variable est continue, sinon on considère des regroupements de modalités pour des variables qualitatives). 

Les arbres de décision ainsi décrits sont simples à obtenir et faciles à interpréter (comme le montre la Figure \ref{cart_titanic} sur les données du Titanic\footnote{Ce jeu de données, contenant des informations sur tous les passagers (et membres d'équipage) du Titanic, dont la variable $y$ indiquant si la personne a survécu a été abondamment utilisé pour illustrer les techniques de classification, voir {\sffamily https://www.kaggle.com/c/titanic/data}.}), mais ils sont peu robustes, et leur pouvoir prédictif est souvent très faible, en particulier si l'arbre est très profond.
Une idée naturelle est de développer un ensemble de modèles d'arbres à peu près indépendants, qui prédisent conjointement mieux qu'un modèle d'arbre unique. On va utiliser le bootstrap, en tirant (avec remise) $n$ observations parmi $\{(\bx_i,y_i)\}$. Ces \revision{ensembles d'arbres - naturellement appelés} « forêts » - une fois agrégés donnent souvent de bien meilleurs résultats que les arbres isolés, mais ils sont difficiles à interpréter. Ces techniques ressemblent toutefois beaucoup à ce qui est fait lorsque l'on utilise les techniques de bootstrap en régression (par exemple pour construire des tubes de confiance dans une régression fonctionnelle).

Le principe du « {\em bagging} », pour « {\em bootstrap aggregating} »,  consiste à générer des échantillons aléatoires, en tirant avec remise dans l'échantillon d'origine, comme pour le bootstrap. Chaque échantillon ainsi généré  permet d'estimer un nouvel arbre de classification, formant ainsi une forêt \revision{d'arbres}. C'est l'agrégation de tous ces arbres qui conduit à la prévision. Le résultat global est moins sensible à l'échantillon initial et donne souvent de meilleurs résultats de prévision.

Les forêts aléatoires, ou « {\em random forests} » \revision{reposent sur} le même principe que le « {\em bagging} », mais en plus, lors de la construction d'un arbre de classification, à chaque branche, un  \revision{sous-}ensemble de $m$ covariables est tiré aléatoirement. Autrement dit, chaque branche d'un arbre ne s'appuie pas sur le même ensemble de covariables. \revision{Cela permet d'amplifier la variabilité entre les différents arbres et d'obtenir, au final, une forêt composée d'arbres moins corrélés les uns aux autres.} 

\subsection{Sélection de modèle de classification}\label{sec:selection:modele}

étant donné un modèle $m(\cdot)$ approchant $\esp[Y\vert \bX=\bx]$, et un seuil $s\in[0,1]$, posons
$$
\widehat{y}^{(s)}=\boldsymbol{1}[m(\bx)>s]
=
\left\lbrace
\begin{array}{l}
1 \text{ si }m(\bx)>s \\
0 \text{ si }m(\bx)\leq s
\end{array}
\right.
$$
La matrice de confusion est alors le tableau de contingence associé aux comptages $\boldsymbol{N}=[N_{u,v}]$ avec
$$
N_{u,v}^{(s)}=\sum_{i=1}^n \boldsymbol{1}(\widehat{y}^{(s)}_i=u,y_j=v)
$$
pour $(u,v)\in\lbrace0,1\rbrace$. La Table \ref{Tab:confusion} présente un tel tableau, avec le nom de chacun des éléments : TP ({\em true positive}) sont les vrais positifs, correspondant aux $1$ prédits en $1$, 
TN ({\em true negative}) sont les vrais négatifs, correspondant aux $0$ prédits en $0$, FP ({\em false positive}) sont les faux positifs, correspondant aux $0$ prédits en $1$, et enfin FN ({\em false negative}) sont les faux négatifs, correspondant aux $1$ prédits en $0$).

\begin{table}
\begin{center}
\begin{tabular}{|c|cc|c|}\hline
                & $y=0$ & $y=1$ & \\ \hline
$\widehat{y}_s=0$ &  {TN}${}_s$   & {FN}${}_s$     & TN${}_s$+FN${}_s$ \\
$\widehat{y}_s=1$ &  {FP}${}_s$   & {TP}${}_s$     & FP${}_s$+TP${}_s$ \\ \hline
                &  TN${}_s$+FP${}_s$   & FN${}_s$+TP${}_s$    & $n$ \\ \hline
\end{tabular}
\end{center}
\caption{Matrice de confusion, ou tableau de contingence pour un seuil $s$ donné.}\label{Tab:confusion}
\end{table}

Plusieurs quantités sont dérivées de ce tableau. La sensibilité correspond à la probabilité de prédire $1$ dans la population des $1$, ou taux de vrais positifs. La spécificité est  la probabilité de prédire $0$ dans la population des $0$ ou taux de vrais négatifs. On s'intéressera toutefois davantage au taux de faux négatifs,  c'est à dire la probabilité de prédire $1$ dans la population des $0$. La représentation de ces deux valeurs lorsque $s$ varie donne la courbe ROC (« {\em receiver operating characteristic} ») :
$$
\text{ROC}_s=\left(\frac{\text{FP}_s}{\text{FP}_s+\text{TN}_s},\frac{\text{TP}_s}{\text{TP}_s+\text{FN}_s}\right)=(\text{\sf sensibility}_s,1-\text{\sf specificity}_s) \text{ pour }s\in[0,1].
$$
Une telle courbe est présentée dans la partie suivante, sur des données réelles.

Les deux grandeurs intensivement utilisées en apprentissage automatique sont l'indice $\kappa$, qui compare la précision observée avec celle espérée, avec un modèle aléatoire (tel que décrit dans \cayNP{LandisKoch}) et l'AUC correspondant à l'aire sous la courbe ROC. Pour le premier indice, une fois choisi $s$, notons $\boldsymbol{N}^\perp$ le tableau de contingence correspond aux cas indépendants (défini à partir de $\boldsymbol{N}$ dans le test d'indépendance du chi-deux).
On pose alors
$$
\text{précision totale}=\frac{\text{TP+TN}}{n}%
$$
alors que
$$
\text{précision aléatoire}=\frac{[\text{TN+FP}]\cdot[\text{TP+FN}] 
+[\text{TP+FP}]\cdot[\text{TN+FN}]}{n^2}
$$
On peut alors définir
$$
\kappa=\frac{\text{précision totale}-\text{précision aléatoire}}{1-\text{précision aléatoire}}
$$
Classiquement $s$ sera fixé égal à 0.5, comme dans une classification Bayésienne naïve, mais d'autres valeurs peuvent être retenues, en particulier si les deux erreurs ne sont pas symétriques (nous reviendrons sur ce point dans un exemple par la suite).

Il existe des compromis entre des modèles simples et complexes mesurés par leur nombre de paramètres (ou plus généralement les degrés de liberté) en matière de performance et de coût. Les modèles simples sont généralement plus faciles à calculer, mais peuvent conduire à des ajustements plus mauvais (avec un biais élevé par exemple). Au contraire, les modèles complexes peuvent fournir des ajustements plus précis, mais risquent d'être coûteux en termes de calcul. En outre, ils peuvent surpasser les données ou avoir une grande variance et, tout autant que des modèles trop simples, ont de grandes erreurs de test. Comme nous l'avons rappelé auparavant, dans l'apprentissage machine, la complexité optimale du modèle est déterminée en utilisant le compromis de biais-variance.

\subsection{De la classification à la régression}

Comme nous l'avons rappelé en introduction, historiquement, les méthodes d'{apprentissage automatique} se sont orientées autour des problèmes de classification (avec éventuellement plus de 2 modalités\footnote{Par exemple dans le cas de  reconnaissance de lettres ou de chiffres.}), et assez peu dans le cas où la variable d'intérêt $y$ est continue. Néanmoins, il est possible d'adapter quelques techniques, comme les arbres et les forêts aléatoires, le boosting, ou les réseaux de neurones.

Pour les arbres de régression, \cayNP{Morganetal} ont proposé la méthode AID, basée sur la formule de décomposition de la variance de l'équation (\ref{eq:pyt}), avec un algorithme proche de celui de la méthode CART décrite auparavant. Dans le contexte de la classification, on calculait, à chaque n\oe{}ud (dans le cas de l'indice \revision{d'impureté} de Gini) en sommant sur la feuille de gauche $\{x_{k,i}<s\}$ et celle de droite $\{x_{k,i}>s\}$
$$
I=\sum_{i:x_{k,i}<s} \overline{y}_{\text{g}} \big(1-\overline{y}_{\text{g}}\big)
+\sum_{i:x_{k,i}>s} \overline{y}_{\text{d}} \big(1-\overline{y}_{\text{d}}\big)
$$
où $\overline{y}_{\text{g}}$ et $\overline{y}_{\text{d}}$ désignent les fréquences de $1$ dans la feuille de gauche et de droite, respectivement. Dans le cas d'un arbre de régression, on utilisera
$$
I=\sum_{i:x_{k,i}<s} \big(y_i-\overline{y}_{\text{g}}\big)^2
+\sum_{i:x_{k,i}>s}  \big(y_i-\overline{y}_{\text{d}}\big)^2
$$
qui va correspondre à la somme (pondérée) des variances intra. Le partage optimal sera celui qui aura le plus de variance intra (on veut les feuilles les plus homogènes possibles) ou de manière équivalente, on veut maximiser la variance intra.

Dans le contexte des forêts aléatoires, on utilise souvent un critère majoritaire en classification (la classe prédite sera la classe majoritaire dans une feuille), alors que pour la régression, on utilise la moyenne des prédictions, sur tous les arbres.

%\subsection{La notion d'apprentissage}


Dans la partie précédente, nous avons présenté la dimension « apprentissage » de l'apprentissage automatique en présentant le « {\em boosting} ». Dans un contexte de régression (variable $y$ continue), l'idée est de créer une succession de modèles en écrivant l'équation (\ref{eqboot}) sous la forme :
$$
m^{(k)}(\boldsymbol{x})=m^{(k-1)}(\boldsymbol{x})+\alpha_k \underset{h\in\mathcal{H}}{\text{argmin}}\left\lbrace \sum_{i=1}^n (y_i,m^{(k-1)}(\boldsymbol{x})+h(\boldsymbol{x}))^2\right\rbrace
$$
où $\alpha_k$ est un paramètre de « {\em shrinkage} », où le second terme correspond à un arbre de régression, sur les résidus, $y_i-m^{(k-1)}(\boldsymbol{x}_i)$.

Mais il existe d'autres techniques permettant d'apprendre de manière séquentielle. Dans un modèle additif ({\sc gam}) on va chercher une écriture de la forme
$$
m(\boldsymbol{x})=\sum_{j=1}^p m_j(x_j)=m_1(x_1)+\cdots+m_p(x_p)
$$
L'idée de la poursuite de projection repose sur une décomposition non pas sur les variables explicatives, mais sur des combinaisons linéaires. On va ainsi considérer un modèle
$$
m(\boldsymbol{x})=\sum_{j=1}^k g_j(\boldsymbol{\omega}_j\transpose\boldsymbol{x})=g_1(\boldsymbol{\omega}_1\transpose\boldsymbol{x})+\cdots+g_k(\boldsymbol{\omega}_k\transpose\boldsymbol{x}).
$$
Tout comme les modèles additifs, les fonctions $g_1,\cdots,g_k$ sont à estimer, tout comme les directions $\boldsymbol{\omega}_1,\cdots,\boldsymbol{\omega}_k$. Cette écriture est relativement générale, et permet de tenir compte d'interactions et d'effets croisés (ce que nous ne pouvions pas faire avec les modèles additifs qui ne tiennent compte que de non-linéarités). Par exemple en dimension 2, un effet multiplicatif $m(x_1,x_2)=x_1\cdot x_2$ s'écrit
$$
m(x_1,x_2)=x_1\cdot x_2=\frac{(x_1+x_2)^2}{4}-\frac{(x_1-x_2)^2}{4}
$$
autrement dit $g_1(x)=x^2/4$, $g_1(x)=-x^2/4$, $\boldsymbol{\omega}_1=(1,1)\transpose$ et $\boldsymbol{\omega}_1=(1,-1)\transpose$. Dans la version simple, avec $k=1$, avec une fonction de perte quadratique, on peut utiliser un développement de Taylor pour approcher $[y_i-g(\boldsymbol{\omega}\transpose\boldsymbol{x}_i)]^2$, et construire classiquement un algorithme itératif. Si on dispose d'une valeur initiale $\boldsymbol{\omega}_0$, notons que
$$
\sum_{i=1}^n[y_i-g(\boldsymbol{\omega}\transpose\boldsymbol{x}_i)]^2
\approx 
\sum_{i=1}^n g'(\boldsymbol{\omega}_0\transpose\boldsymbol{x}_i)^2\left[\boldsymbol{\omega}\transpose\boldsymbol{x}_i+\frac{y_i-g(\boldsymbol{\omega}_0\transpose\boldsymbol{x}_i)}{g'(\boldsymbol{\omega}_0\transpose\boldsymbol{x}_i)}-
\boldsymbol{\omega}\transpose\boldsymbol{x}_i\right]^2
$$
qui correspondrait à l'approximation dans les modèles linéaires généralisés sur la fonction $g(\cdot)$ qui était la fonction de lien (supposée connue). On reconnaît  un problème de moindres carrés pondérés. La difficulté ici est que les fonctions $g_j(\cdot)$ sont inconnues.
