# Supplementary material for: Applying Machine Learning to Life Insurance: some knowledge sharing to master it
Source: arXiv:2209.02057 source file (2022-09-27)
Supplement: Supplementary file 2 [file algo_sourceDimitri.tex]

\subsubsection{Algorithme CART}
Pour expliquer les arbres de décision de manière globale, nous nous plaçons dans le cas simplifié d'arbres de classification binaires. La méthode présentée se généralise pour les arbres de régression.
Nous présentons l'algorithme le plus couramment utilisé, c'est-à-dire celui présenté par Breiman et Al. en 1984 [\ref{brieman}].\\
Soit $Y \in \{1,...,K\}$ la variable catégorielle que l'on cherche à expliquer et $X  \in \mathds{R}^p$ ($p,K \in \mathds{N}$).
On suppose que l'on dispose d'un échantillon: $y=(y_1,...,y_n) \in \mathds{R}^n$ correspondant aux valeurs cibles et $x=(x_{ij})_{1 \leq i \leq n, 1 \leq j \leq p}$ correspondant aux variables explicatives (avec $n \in \mathds{N}$ le nombre d'individus).


\paragraph{Principe général\\}
Un arbre binaire est obtenu en séparant les individus successivement en deux sous-ensembles. L'objectif à chaque étape est de trouver la variable explicative qui sépare le mieux possible les données en deux sous-groupes. On s'arrête lorsque une nouvelle division ne nous apporte pas d'amélioration ou lorsqu'un sous-groupe est trop petit.
On note déjà  que la construction d'un arbre nécessite : un processus de sélection des divisions successives de l'arbre, d'un critère pour décider de réaliser une nouvelle coupe ou de considérer le noeud comme terminal et d'un processus d'attribution de classe à chaque noeud terminal (ou feuille).

\paragraph{Notations utilisées\\}
Nous utiliserons pour la suite les notations suivantes:
\begin{itemize}
    \item $I$ l'ensemble des individus et $i \in I$ un individu. 
    \item $C$ une partition de l'échantillon, et $t \in C$ un noeud
    \item $N(t)$: le nombre d'individus dans un noeud $t$.
    \item $N_k(t)$: le nombre d'individus de classe $k$ dans le noeud t.
    \item $p(k|t)=\frac{N_k(t)}{N(t)}$ la proportion d'individus de classe k dans le noeud t.
    \item $y(t)$ la prédiction faite pour les individus du noeud t: on choisit la classe majoritaire, i.e: $y(t)=j <=>\forall k \in K, p(k|t) \leq p(j|t)$ (en régression on utiliserait une moyenne pondérée).
\end{itemize}
\paragraph{Construction de l'arbre maximal\\}
La première partie de l'algorithme CART consiste à créer un arbre, dit maximal.
\subparagraph{Fonction d'impureté : }
Définissons tout d'abord la notion d'impureté. Un noeud est dit pur si une seule classe est représentée dans le noeud.
L'objectif est d'introduire une fonction qui renvoyant un réel positif, donnant le degré d'impureté du noeud. Ainsi pour un noeud t donné, on définit la fonction $Imp$ telle que:
\begin{equation}\phi: [0,1]^K \rightarrow \mathds{R}, Imp(t)= \phi(\{p(k|t), k \in K\})
\end{equation}
Cette fonction $\phi$, positive, doit vérifier les conditions suivantes:
\begin{itemize}
    \item elle prend son maximum uniquement lorsque les classes sont équiréparties, c'est-à-dire au point: $(\frac{1}{K},...,\frac{1}{K})$
    \item elle prend son minimum lorsque le noeud est pur, c'est-à-dire pour tous les points contenant K-1 zéro et un unique 1.
    \item elle est symétrique, c'est-à-dire qu'elle ne privilégie pas une classe plus qu'une autre
\end{itemize}
L'exemple le plus classique d'impureté est la fonction d'entropie définie par:
\begin{equation}Ent(t)=\sum\limits_{k \in K}{p(k|t)\ log\ p(k|t)}\end{equation}
\begin{equation}Gini(t)=\sum\limits_{k=1}^{K}{p(k|t)(1-p(k|t))}\end{equation}
\subparagraph{Division d'un noeud :}
Soit $x_j (j \in \{1,...,p\}) $la variable que l'on souhaite utiliser pour créer une coupe à partir d'un noeud $t$ donné, pour former deux sous-noeuds: $t_G$ et $t_D$. Dans le cas de variables quantitatives,on chercherait un réel $z$ qui sépare au mieux le noeud en deux sous-noeuds:
$t_G(z)=\{w \in t, x_j(w) \leq z\}$ et $t_D(z)=\{w \in t, x_j(w) > z\}$.
On cherche z qui minimise la fonction:

\begin{equation}z \mapsto \Delta Imp(d_z(t),t) = Imp(t) - \frac{N(t_G(z))}{N(t)}Imp(t_G(z)) - \frac{N(t_D(z))}{N(t)}Imp(t_D(z))\end{equation} où $d_z(t)$ est la division du noeud $t$ associée au réel $z$.
On cherche à maximiser l’homogénéité des noeuds obtenus, un noeud étant parfaitement homogène s’il ne
contient que des individus de la même classe.
Dans le cas de la régression, on cherche à créer des découpes qui tendent à diminuer la variance des noeuds.
Nous disposons à présent de l'algorithme pour créer l'arbre maximal: à partir de la racine de l'arbre (un arbre vide initialement), on réalise une découpe en utilisant le critère de division de noeud vu précédemment. Sur chacun des sous-noeuds ainsi formés on met en place le processus, et ainsi de suite. Deux conditions supplémentaires sont ajoutées pour fixer l'arrêt de l'algorithme: \begin{itemize}
    \item On introduit un critère d'arrêt qui impose de ne pas découper un noeud qui contient moins d'un certain nombre d'individu.
    \item On ne découpe pas un noeud pur, c'est-à-dire qu'un noeud pur est nécessairement une feuille de l'arbre.
\end{itemize}

Ainsi à la fin de cet algorithme, on a créé l'arbre maximal noté $T_{max}$. Cependant, ce n'est pas nécessairement cet arbre que l'on va utiliser pour la prédiction, mais un sous-arbre obtenu en élaguant $T_{max}$.

\paragraph{Élagage de l'arbre maximal\\}
Présentons à présent comment se réalise l'élagage de l'arbre $T_{max}$ construit précédemment.
\subparagraph{Taux d'erreur :}
Définissons pour cela le taux d'erreur, qui sera une notion fondamentale pour comprendre l'élagage.
Au sein d'un noeud t, on le définit ainsi:
\begin{equation}R(t)=\sum\limits_{k \in K,k \neq y(t)}{p(k|t)}\end{equation} 
Il s'agit de la proportion d'individus présents dans le noeud t qui n'ont pas la même valeur cible que la prédiction faite par le noeud t.

On peut alors généraliser cette définition à un arbre et non plus à un unique noeud.  Pour cela, on note $\tau$ l'ensemble des noeuds terminaux (i.e feuilles) de l'arbre T.
On définit alors le taux d'erreur de cet arbre par la formule :
\begin{equation}R(T)=\sum\limits_{t \in \tau}{\frac{N(t) R(t)}{n}}=1-\frac{1}{n} \sum\limits_{t \in \tau}{N_{y(t)}(t)}\end{equation}
Il s'agit de la somme des taux d'erreurs de chaque noeuds terminaux, pondérés par la proportion d'individus au sein de ce noeud.

\subparagraph{Paramètre de complexité et taux d'erreur}
Le taux d'erreur précédemment introduit ne prend pas en compte la complexité de l'arbre. En général, on cherche à ne pas avoir un arbre trop profond, pour éviter le surapprentissage, c'est pourquoi on introduit un terme de pénalité pour favoriser les arbres peu complexes.
On note $\alpha \in \mathds{R^+}$ le paramètre de complexité, et on appelle taux d'erreur pénalisé d'ordre $\alpha$, la fonction $R_{\alpha}$ définie pour un arbre $T$ par:
\begin{equation}
    R_{\alpha}(T)=R(T)+\alpha |T|
\end{equation}
Ainsi, ce nouveau taux pénalise les arbres avec beaucoup de feuilles (paramètre quantifiant la complexité du modèle). 

\subparagraph{Choix de division ou de noeud terminal}
A présent, il nous faut comprendre comment on élague l'arbre. Soit $T$ un arbre, $t$ un noeud de cet arbre, et $T(t)$ le sous-arbre de $T$ issu du noeud $t$. On a nécessairement $R(T(t)) \leq R(t)$. Pour savoir si on élague, pour un paramètre de complexité $\alpha$ donné, l'élagage est utile si le taux d'erreur (pénalisé) du sous-arbre $T(t)$ est plus grand que le taux d'erreur (pénalisé) du noeud t, c'est-à-dire si: $R_{\alpha}(T(t)) \geq R_{\alpha}(t)$. 
De plus, $$R_{\alpha}(T(t)) \geq R_{\alpha}(t)\ <=>\ R(T(t)) + \alpha |T(t)| \geq R(t) + \alpha \ <=> \ \alpha \leq \frac{R(t)-R(T(t))}{|T(t)|-1}$$
On note la fonction introduite ci-dessus $g: g(t,T)=\frac{R(t)-R(T(t))}{|T(t)|-1}$.
On appelle alors maillon faible $t_{min}$, le noeud qui minimise cette fonction:
$t_{min}=\underset{t \in T}{argmin} \ g(t,T)$. Le paramètre de complexité choisi est alors: $\alpha=g(t_{min},T)$.

\subparagraph{Algorithme d'élagage}
La paragraphe précédent nous fournit alors un algorithme bottom-up d'élagage, qui va renvoyer une liste d'arbres élagués issus de $T_{max}$:
\begin{itemize}
    \item Entrée: arbre maximal $T_{max}$ construit précédemment
    \item Initialisation: $\alpha_0=0$, $T_0=Tmax, k=0$
    \item Itération: Tant que $|T_{max}|>1$:
    \begin{itemize}
        \item $t_{min}^{(k+1)}=\underset{t \in T_k}{argmin \ g(t,T_k)}$ (noeud, correspondant au maillon faible de l'arbre $T_k$)
        \item $\alpha_{k+1}=g(t_{min},T_k)$ (paramètre de complexité)
        \item construction du nouvel arbre $T_{k+1}$ à partir de $T_k$ en élaguant toutes les branches issues de $t_{min}^{k+1}$ 
    \end{itemize}
    \item Outputs: $\{\alpha_1,...,\alpha_N\}$ et $\{T_{max},T_1,...,T_N\}$ avec $N \in \mathds{N}$ le nombre d'itérations de l'algorithme.
\end{itemize}

L'arbre que l'on retient en général pour la prédiction, est l'arbre $T_k$ pour lequel son taux erreur pénalisé $R_{\alpha_k}(T_k) $ est minimum.
\subsubsection{Importance des variables}
L'importance des variables a été l'une des premières méthodes faisant écho à l'interprétabilité et la transparence d'un modèle. En effet, une question que l'on se pose lorsque l'on ajuste un algorithme de machine learning est : quelles variables ont réellement servi pour la prédiction et quelles sont celles la plus grande contribution ?
La réponse à cette question permet de mieux comprendre le modèle d'une part et de supprimer les variables jugées inutiles d'autre part, en rendant ainsi le modèle plus interprétable par le biais du critère de parcimonie, vu dans le chapitre \ref{chap:def_prop_ML_interpretable}. Brieman fut l'un des premiers à répondre à cette question d'importance des variables, pour le cas des arbres de décision [\ref{brieman}]. Nous verrons dans le chapitre \ref{chap_methodes_interp} une généralisation indépendante du modèle de l'importance des variables, appelée PFI, qui repose sur des permutations entre les différentes variables utilisées dans le modèle.
\paragraph{Division de substitution  \\}
Notons pour tout noeud $t, \ d^*(t)$ la division optimale à partir d'un noeud $t$, c'est-à-dire la division faite au niveau du noeud $t$ au cours de l'algorithme de construction de l'arbre maximal. On note $t_g$ et $t_d$ les sous-noeuds ainsi obtenus. 
Définissons également pour tout $m \in \{1,...,p\}, \ Dm(t)$ l'ensemble des divisions possibles à partir du noeud, en utilisant la variable explicative $x_m$ pour séparer, et $\bar{D_m(t)}$ son complémentaire. Dans le cas de la régression, on aurait des divisions de la forme: $x_m \leq \alpha, \ \alpha \in \mathds{R}$. Pour une division $d_m(t) \in D_m(t)$, on $t_g'$ et $t_d'$ les sous-noeuds ainsi obtenus. 
On note pour tout $j \in\{1,...,K\}$, $N_j(t_g \cap t_g')$ le nombre d'individus de la classe $j$ du noeud $t$ envoyés dans le sous-noeud de gauche par $d_m(t)$ et $d(t)^*$. On utilise les mêmes notations avec l'indice pour les individus envoyés à droite.
Ainsi la probabilité que les divisions $d_m(t)$ et $d^*(t)$ envoient un individu du noeud t dans le sous-noeud de gauche est donnée par:
\begin{equation}p_{gg}(d_m(t),d^*(t))= \sum_{k=1}^{K}{\frac{p(k|t) N_j(t_g \cap t_g')}{p(t) N_j(t)}}\end{equation}
On a la même définition pour les sous-noeuds droits $p_{dd}(d_m(t),d^*(t))$, avec les indices $d$ à la place de $g$.
On peut alors définir la probabilité que la division $d_m(t)$ prédise correctement la meilleure division $d^*(t)$, par :
$p(d_m(t),d^*(t))=p_{gg}(d_m(t),d^*(t))+p_{dd}(d_m(t),d^*(t))$
La division de substitution $\tilde{d_m}(t)$ associée à une variable explicative $x_m, \ m \in \{1,...,p\}$ est alors définie comme la division $d_m(t) \in D_m(t)$ qui prédit au mieux le partage fait par la division optimale $d^*$, c'est-à-dire:
\begin{equation} \tilde{d_m}(t)= \underset{d_m(t) \in D_m(t)}{argmax} \ p( d_m(t),d^*(t) ) \end{equation}

\paragraph{Définition de l'importance d'une variable\\}
A l'aide des divisions de substitution introduites ci-avant, on peut alors définir l'importance $I_{x_m}$ d'une variable $x_m, \ m \in \{1,...,p\}$, associée à un arbre $T$ par: \begin{equation}I(x_m)=\sum_{t \in T}{\Delta Imp(\tilde{d_m}(t),t)}\end{equation}
Il s'agit de la somme des diminutions de déviance provoquées à chaque noeud $t$ de l'arbre, si on remplaçait la division optimale $d^*(t)$ par la division de substitution $\tilde{d_m}(t)$.
On la normalise en général de sorte à avoir une valeur comprise entre 0 et 1, avec la variable la plus importante fixée à 1.
\paragraph{Stabilité de l'importance des variables CART \\}
Des études empiriques ont été menées par Breiman (1996) et Ghattas (1999) pour montrer l'instabilité des arbres de classification et de régression par rapport à de faibles perturbations des données initiales.
Pour étudier la stabilité de l'importance des variables, on peut utiliser des échantillons \emph{bootstrap} des données d'origine et voir l'impact sur l'importance des variables données pour chaque algorithme CART ajusté.
Ghattas a réalisé cette étude à partir d'une base de données de la station de Vitrolles, afin de prédire le maximum d'ozone dans la station. Les variables explicatives sont nombreuses (39) avec notamment la température, la nébulosité ou encore la quantité de SO2 au sein de la station.
40 échantillons \emph{bootstrap} des données disponibles ont été mis en place, et pour chacun de ces échantillons, un arbre CART de taille fixe (10 feuilles) a été construit.
Pour chaque arbre, l'importance des variables a été calculée, et l'étude de la distribution associée a été réalisée, sous la forme d'une boîte à moustaches, comme nous pouvons le voir sur la figure \ref{fig:cart_imp}.
\begin{figure}[!h]
    \centering
    \includegraphics[width=120mm]{LaTeX_Template_EURIA/Images/Boxplot_imp_var.PNG}
    \caption{Boxplot d'importance de chaque variable, obtenu à partir de 40 arbres construits sur des échantillons \emph{bootstrap} (figure issue de l'article [\ref{CART_stabilite}])}
    \label{fig:cart_imp}
\end{figure}

La variable représentant le maximum d'ozone observé la veille demeure la plus importante sur 39 des 40 échantillons créés, ce qui démontre une stabilité, malgré la perturbation des données. 
Ce n'est pas le cas pour les autres variables importantes telles que le gradient ou la nébulosité qui ont une dispersion significative. 
Les variables les moins importantes semblent elles conserver leur position. 
Finalement, cette analyse a montré une instabilité des variables intermédiaires mais une stabilité des variables peu importantes et très importantes.

\paragraph{Limites de l'importance des variables d'un arbre de décision \\}
L'importance des variables a l'avantage d'être un indicateur simple et facilement compréhensible du comportement du modèle.
Cependant, il devient vite limité et peut donner des résultats extrêmement variables.
Pour mettre en évidence cette limite de l'importance des variables, considérons un problème de classification binaire. On veut mesurer l'importance de deux variables $x_1$ et $x_2$ sur la variable à expliquer $y \in \{0,1\}$.
On construit la règle de calcul suivante:
Si $x_1<0.5$ et $x_2<0.5$ ou $x_1 \geq 0.5$ et $x_2 \geq 0.5: \ y=0$, sinon $y=1$.
On construit un échantillon de taille $n=1000$ défini suivant cette règle, avec $x_1$ et $x_2$ suivant une loi uniforme sur $[0,1]$,

Pour cet échantillon de taille 1000, nous ajustons un arbre de décision, avec la fonction \emph{rpart} de R, en utilisant les paramètres de base. A l'aide de cet ajustement, nous calculons l'importance des variables $x_1$ et $x_2$.
Nous répétons cette opération $N=1000$ fois et nous analysons la distribution de l'importance des variables observées (pour la variable $x_1$ par exemple). Pour se faire, nous normalisons l'importance des variables de sorte à avoir une valeur entre 0 et 100. 

\begin{figure}[!h]
\begin{tabular}{ccc}
\centering

\includegraphics[width=80 mm]{LaTeX_Template_EURIA/Images/limite_imp_var_ggplot.jpeg} &\includegraphics[width=80 mm]{LaTeX_Template_EURIA/Images/exemple_arbre_decision.png} & \\
\includegraphics[width=80 mm]{LaTeX_Template_EURIA/Images/imp_var_densite.png}
\end{tabular}
\caption{Mise en place d'un modèle CART sur des données simulées afin de montrer la limite de l'importance des variables}
\label{fig:limite_var_imp}
\end{figure}
Nous observons très clairement que dans la plupart des cas, l'importance estimée par le modèle n'est pas de 50\%, comme on aurait pu le penser intuitivement.
Dans la majorité des cas, il surestime l'importance d'une variable au détriment de l'autre. Ainsi, il faut se méfier de la notion d'importance des variables, et ne s'interprète pas aussi intuitivement qu'on ne le croit.




\subsubsection{Interprétabilité des arbres de décision}
Les arbres de décision font partie de la classe d'algorithmes considérés comme "interprétables". En effet, leur structure simple d'arbre leur permet d'expliquer facilement les prédictions réalisées. L'arborescence nous invite à raisonner de manière "contrefactuelle", c'est-à-dire que pour comprendre une prédiction d'une certaine instance, on se demande l'impact sur la décision si une variable avait été inférieure ou supérieure à une certaine valeur, ou si elle changeait de catégorie. 
Ceci peut être vu sur l'exemple simple des données Titanic \footnote{Données Titanic disponibles sur : \url{https://gist.github.com/michhar/2dfd2de0d4f8727f873422c5d959fff5}.} dont l'objectif est de prédire la survie ou non d'un individu en fonction de ses caractéristiques, dont l'âge. 
Supposons que l'on obtient le modèle décrit sur la figure \ref{fig:cart_titanic}. Alors il est facile d'interpréter les prédictions faites. En effet, si un individu est un homme de 30 ans, alors sa probabilité de survie estimée par le modèle est de 17 \%. Si cet individu avait été une femme alors sa probabilité de survie estimée par le modèle aurait été de 74 \%, tandis que si il avait été âgé de moins de 6 ans et demi, alors elle aurait été de 67 \%.
\\
\begin{figure}[!h]
    \centering
    \includegraphics[width=90mm]{LaTeX_Template_EURIA/Images/CART_titanic.png}
    \caption{Modèle d'arbre de décision sur la probabilité de survie d'un passager du Titanic en fonction de son âge et de son sexe}
    \label{fig:cart_titanic}
\end{figure}
\\
Cette simplicité d'interprétation en fait l'un des modèles de data science les plus prisés comme alternative aux méthodes traditionnelles (statistiques univariées, bivariées, etc.). Il peut également servir comme modèle de substitution à un modèle plus complexe comme nous le verrons dans l'annexe \ref{annexe:mod_sub_global}.
%\section{Règles de décision et algorithme RuleFit}







%\chapter[Modèles complexes]{Modèles complexes}
%\thispagestyle{empty}

\section{Un exemple de modèle complexe : XGBoost}
Dans cette partie, on s'intéresse à un modèle de Machine Learning en particulier : le XGBoost.
Celui-ci utilise de manière judicieuse les arbres de décisions, détaillés ci-avant, pour former un modèle plus complexe et généralement plus performant.
Il est désormais largement utilisé dans de nombreux domaines, y compris en actuariat, notamment pour ses nombreux hyperparamètres que l'on peut régler le plus finement possible pour améliorer la précision.
Ce modèle sera utilisé dans notre application actuarielle du chapitre \ref{chap:application_tarif}, notamment pour la modélisation fréquentielle en tarification automobile. Considéré comme boîte-noire, le XGBoost sera alors interprété à l'aide des outils développés au cours du chapitre \ref{chap_methodes_interp}.  

D'autres algorithmes d'apprentissage statistiques jugés complexes ont été envisagés lors de notre application et sont détaillés en annexe \ref{annexe:nnet_svm}.

\subsection{Boosting}
Pour comprendre l'algorithme XGBoost, il est nécessaire de rappeler le Boosting et notamment Adaboost, ainsi que l'algorithme de Gradient Boosting. 
Le Boosting est une technique ensembliste qui consiste à agréger des classifieurs faibles \footnote{Le terme de classifieur faible (\emph{weak classifier}) proposé par Shapire [\ref{adaboost}] fait référence à un modèle légèrement plus performant que le modèle trivial.} qui sont construits étape par étape, en corrigeant au fur et à mesure les poids des individus [\ref{adaboost}].  L'objectif est alors d'obtenir un classifieur fort \footnote{Par opposition au classifieur faible, un classifieur fort fait écho à un modèle bien plus performant que le modèle trivial. [\ref{adaboost}]}.

Description de l'algorithme de Boosting (Adaboost):
Soit $B$ le nombre de modèles utilisés, $(ALGO)$ l'algorithme utilisé (par exemple un arbre de décision), $y$ la variable binaire cible : $y \in \{-1,1\}$, $X$ la matrice des variables explicatives.
On considère l'ensemble d'apprentissage que l'on a à notre disposition: 
$(x_1,y_1),...,(x_n,y_n)$, c'est-à-dire: $x=(x_{i,j})_{1 \leq i \leq n, 1 \leq j \leq p}$ et $(y_{i})_{1 \leq i \leq n }$

\begin{itemize}
    \item $LISTE$, une liste qui contiendra les différents modèles et initialement vide. %$\varnothing$ 
    \item les individus sont pondérés uniformément: $w_i^1=1/n$
    \item pour $b = 1$ à $B$:
    \begin{itemize}
        \item construire le modèle $M_b$ reposant sur les données pondérées par $w^b=(w_i^b)_{\{1\leq i\leq n\}}$ à l'aide de $(ALGO)$. On note $\hat{y_i} = M_b(x_i)$ la prédiction faite par le modèle $M_b$.
        \item ajouter $M_b$ dans $LISTE$
        \item calcul du taux d'erreur commis par $M_b$: $\epsilon_b=\sum\limits_{i=1}^{n}{w_i \mathds{I}_{\{y_i \neq \hat{y_i}\}}}$
        \item si $ \epsilon_b >0.5$ ou $\epsilon_b=0$: arrêt de l'algorithme 
        \item sinon:
        \begin{itemize}
            \item calcul du poids du classifieur: $\alpha_b=ln(\frac{1-\epsilon_b}{\epsilon_b})$
            \item calcul du poids suivant: $w_i^{b+1}=w_i^b e^{\alpha_b \mathds{I}_{\{y_i \neq \hat{y_i}\}}}$
        \end{itemize}
    \end{itemize}
\end{itemize}

A la fin de cet algorithme, un vote pondéré par $(\alpha_b)_{1 \leq b \leq B}$ est ensuite effectué et finalement:
\begin{equation}f(x) = sign(\sum\limits_{b=1}^{B}{\alpha_b M_b(x)})\end{equation} où $x$ est le vecteur des variables explicatives d'entrée, et $f(x)$ la sortie estimée par notre modèle de Boosting.
Il existe de nombreuses variantes sur le choix des poids $\alpha$ des classifieurs.
Nous voyons ici que nous avons le choix sur le type de modèle utilisé (c.f. $(ALGO)$). En général, ce sont des arbres de décision qui sont utilisés car ils permettent de remplir le critère de classifieur faible.
\subsubsection{Algorithme d'optimisation de descente de gradient}
Pour faire le lien avec l'algorithme de gradient boosting, il est nécessaire de rappeler l'algorithme de descente de gradient. Ce dernier est une technique itérative qui permet d'approcher la solution d'un problème d'optimisation convexe .
Considérons une fonction deux fois différentiable $f$, d'espace de départ $\mathds{R}^p$ (muni de la norme $\parallel .\parallel $ et du produit scalaire $<.>$) et d'espace d'arrivée $\mathds{R}$, qu'on souhaite minimiser. Pour $x \in \mathds{E}$, on note $\nabla f(x)$ le gradient de $f$ en $x$: $\nabla f(x)=(\frac{\partial f}{\partial x_i}(x))_{1 \leq i \leq p}$.
On choisit une valeur initiale $x_0 \in \mathds{R}^p$ pour l'algorithme, ainsi qu'un seuil (critère d'arrêt) $\epsilon > 0$. L'algorithme va alors calculer de manière itérative des valeurs $x_1, x_2,...$ jusqu'à la convergence vers l'optimum. 
L'algorithme est le suivant:
\begin{itemize}
    \item k=0
    \item tant que $ \parallel \nabla f(x_k) \parallel > \epsilon $:
        $x_{k+1}= x_k - \alpha_k \nabla f(x_k)$, avec $\alpha_k$ un paramètre calculé à chaque itération ou bien un paramètre constant $\alpha$.
\end{itemize}

Cet algorithme utilise le fait qu'une fonction décroît plus fortement autour d'un point $x$ dans le sens opposé au gradient, ce qui justifie le signe moins dans la formule itérative précédente.

Appliquons à présent cet algorithme d'optimisation à la fonction coût du modèle considéré.
Notons $j$ notre fonction de coût utilisée pour comparer la valeur $f(x_i)=\hat{y_i}$ prédite par notre modèle et la valeur $y_i$ réelle  (par exemple $j(y_i,f(x_i))=(y_i-f(x_i))^2$ couramment utilisée en régression).
Notons $J$ la fonction de coût global, définie comme la somme des fonctions de coût individuelles: $J(y,f)=\sum\limits_{i=1}^{n}{j(y_i,f(x_i)}$
L'objectif va être alors de minimiser cette fonction de coût, par rapport aux paramètres de la fonction $f$ associée à notre modèle, à l'aide de la méthode de descente du gradient vu précédemment.
Ainsi, si on note $f_b$ notre classifieur à l'étape b de l'algorithme, nous obtenons la formule suivante :
\begin{align} f_b(x)& =f_{b-1}(x)-\alpha \nabla j(y,f(x)) \\ &=f_{b-1}(x_i)-\alpha \frac{\partial j(y_i,f(x_i))}{\partial f(x_i)}, 1 \leq i \leq n \end{align}

On remarque alors que l'algorithme de Boosting présenté au-dessus consiste à optimiser une fonction de coût, à l'aide de la méthode de descente de gradient avec une fonction de coût exponentielle.
En reprenant notre exemple avec $y \in \{-1,1\}$ notre variable à expliquer, et en notant $f$ notre classifieur agrégé à partir des modèles individuels $M_1, M_2, ...$:
$J(f)=\sum\limits_{i=1}^{n}{exp(-y_i f(x_i))}$ (notre fonction de coût à minimiser).

\subsubsection{Algorithme de Gradient Boosting}
\paragraph{Cas de la régression \\}
Nous pouvons à présent définir la méthode de Gradient Boosting, qui généralise l'approche précédente, avec d'autres fonctions de coût.
Les notations précédentes sont conservées, à savoir $f_i$ pour les fonctions associées au modèle de l'itération $i$, $J$ la fonction de coût.
L'algorithme se présente ainsi:
\begin{itemize}
    \item initialisation par un modèle constant: $f_0(x)=\underset{\theta}{\mathrm{argmin}} \sum\limits_{i=1}^{n}{J(y_i,\theta)}$ (correspondant à la moyenne des observations de y pour une fonction de coût correspondant à la norme euclidienne)
    \item pour $m$ allant de $1$ à $M$ (on pourrait aussi introduire un critère d'arrêt):
    \begin{itemize}
        \item calul des pseudo résidus: $r_{i,m}=-\frac{\partial J(y_i,f(x_i)}{\partial f(x_i)}|_{f(x)=f_{m-1}(x)}, 1 \leq i \leq n$
        \item ajustement d'un classifieur $h_m(x)$ (faible, comme un arbre par exemple), entraîné sur les données $(x_i,r_{i,m})_{1 \leq i \leq n}$, où $(x_i)_{1 \leq i \leq n}$ sont les variables explicatives et $(r_{i,m})_{1 \leq i \leq n}$ les sorties.
        \item calcul du prochain classifieur: $f_m(x)=f_{m-1}(x) + \theta_m h_m(x)$, où $\theta_m$ est obtenu en résolvant le problème d'optimisation: $\theta_m=\underset{\theta}{\mathrm{argmin}} \sum\limits_{i=1}^{n}{J(y_i,f_{m-1})(x)+
        \theta h_m(x_i)}$
    \end{itemize}
\end{itemize}
A la sortie de cet algorithme, on obtient: $f_M(x)$ qui est notre classifieur final.
Les fonctions de coûts généralement choisies pour la régression sont:
\begin{itemize}
    \item \textit{écart quadratique}: $j(y_i,f(x_i))=\frac{1}{2}(y_i - f(x_i))^2$. Cette fonction présente l'avantage d'être sensible aux écarts mais l'inconvénient d'être peu robuste vis à vis des points aberrants
    \item \textit{valeur absolue}: $j(y_i,f(x_i))=|y_i-f(x_i)|$. L'avantage de ce choix réside dans sa robustesse aux points abérrants mais est moins sensible aux écarts
    \item \textit{fonction Huber}: $j(y_i,f(x_i))= \left\{\begin {matrix}
y_i-f(x_i)\ si \ |y_i-f(x_i)| < \delta_q \\ 
\delta_q sign(y_i - f(x_i)) \ sinon
\end{matrix}\right.$  où $\delta_q$ est le quantile d'ordre q de $(|y_i-f(x_i)|)_{1 \leq i \leq n}$. 
Ceci permet d'obtenir les avantages de la valeur absolue (sensibilité aux valeurs faibles du gradient) et de l'écart quadratique (sensibilité aux valeurs élevées du gradient).

\end{itemize}



\paragraph{Cas de variable cible catégorielle \\}
Dans le cas où la variable cible est catégorielle avec K modalités (de 1 à K), l'algorithme reste très proche de celui présenté précédemment, avec néanmoins une fonction de coût différente, adaptée au classement.
Pour cela on définit: $$y_i^k= \left\{\begin {matrix}
1 \ si \ y_i=k \\ 
0 \ sinon
\end{matrix}\right., 1 \leq i \leq n, 1 \leq k \leq K$$
La nouvelle fonction de coût est alors définie par:
\begin{equation}j(y_i,f(x_i))=-\sum\limits_{k=1}^{K}{y_i^k log(p^k(x_i))}\end{equation} où $p_k(x_i)$ correspond à la probabilité conditionnelle d'appartenir à la classe k, i.e: \begin{equation}p_k(x_i)=\frac{exp(f^k(x_i))}{\sum\limits_{k=1}^{K}{exp(f^k(x_i))}}
\end{equation}
On travaille donc à présent sur les indicatrices ($y^k$), et on construit des modèles (généralement des arbres) sur les gradients négatifs pour les K classes. $f^k$ est ainsi le modèle additif issu des K modèles précédents.

\subsubsection{Tree Gradient Boosting}
Le Tree Gradient Boosting est le cas particulier du Gradient Boosting où les modèles $h_m$ choisis sont des arbres de décision. Les  paramètres à optimiser peuvent alors être les poids $w_j$ à chaque feuille, ainsi que le nombre de feuilles $T$ dans chaque arbre.
Le XGBoost présenté ensuite est une implémentation plus rapide de cet algorithme.

%\subsection{Mécanismes de régularisation}
%Afin de faire face au surapprentissage auquel sont confrontés les méthodes citées précédemment, différentes méthodes de régularisation existent afin d'essayer d'y remédier.

%\subparagraph{Shrinkage}
%\subparagraph{Gradient Boosting Stochastique}


\subsection{XGBoost}
XGBoost est une manière optimisée et plus rapide de réaliser l’algorithme de Tree Gradient Boosting. Ce dernier est un algorithme d'apprentissage supervisé qui tente de prédire le plus précisément possible une variable cible, en combinant de manière séquentielle les prédictions de plusieurs algorithmes dits faibles. Le plus souvent, on utilise des arbres de décisions avec peu de noeuds comme apprenants faibles (\emph{weak learners}).
Le fait de travailler de manière séquentielle le différencie des forêts aléatoires et le rend plus lent mais lui permet de s'améliorer au fur et à mesure.
L'algorithme tente d'optimiser à chaque itération une fonction objective régularisée (en norme $\mathds{L}^1$ et $\mathds{L}^2$), constituée d'une fonction de coût et d'un terme de pénalité pour tenir compte de la complexité du modèle. A chaque itération, le nouveau modèle prédit la partie résiduelle que l'on n'a pas su expliquer à l'itération précédente. L'output est alors la somme des prédictions faites par chaque modèle.
Le terme de Gradient Boosting vient du fait que la méthode utilisée pour l'optimisation à chaque étape est une descente de gradient.\\

L'intérêt du XGBoost réside dans la correction d’un problème majeur du Tree Gradient Boosting, à savoir le fait de considérer la perte potentielle pour chaque séparation possible (\emph{split}) à un noeud donné pour créer une nouvelle branche. En effet, dans le cas où nous disposons de beaucoup de variables explicatives, il y a un grand nombre de splits possibles, ce qui engendre des temps de calcul élevés.\\

Notons que nous allons présenter l'algorithme uniquement dans le cadre de la régression, mais celui-ci s'adapte pour la classification.

\subsubsection{Algorithme}
Considérons un problème de régression pour lequel nous voulons prédire la variable $Y \in \mathds{R}$, à partir d'un vecteur $X$ de $p$ variables explicatives: $X \in \mathds{R^p}$ ($p \in \mathds{N}$).
Nous reprenons les idées du Boosting, à savoir agréger les prédictions de plusieurs classifieurs dits faibles pour former un classifieur fort.

\paragraph{Entraînement séquentiel \\}
Soit B le nombre d'étapes de notre algorithme. 
Notons pour $b \in \{1,...,B\}$: 
\begin{itemize}
    \item $H$ l'ensemble des modèles sur lequel on va réaliser l'optimisation
    \item $j:\mathds{R}$x$\mathds{R} \rightarrow \mathds{R}$ une fonction de coût choisie au préalable (comme le MSE par exemple).
    \item $\hat{h}_b:\mathds{R}^p$ x $\mathds{R}^n$ $ \rightarrow \mathds{R}^n$ la fonction associée au modèle $M_b$ de l'étape $b$ de l'algorithme, renvoyant le vecteur de prédiction de l'input. Notons bien que le modèle $M_b$ apprend sur les valeurs résiduelles à l'étape b et non la valeur de y.
    \item $\hat{y}^{(b)}$ notre estimation de y à l'étape b.
    \item $r^{(b)}$ le vecteur de taille n des pseudo-résidus au début de l'étape b, c'est-à-dire la partie résiduelle de la valeur cible initiale que nous n'avons  pas encore réussi à expliquer avant l'itération b: $r^{(b)}=y - \hat{y}^{(b-1)} $ et $r^{(0)}=\hat{y}^{(0)}$
    \item $\hat{r}^{(b)}$ l'estimation du vecteur $r^{(b)}$ faite par l'algorithme $M_b$ à l'étape b, soit: $\hat{r}^{(b)}=\hat{h}_b(x)$.
\end{itemize} 
On peut résumer ceci par les relations suivantes:  \begin{equation}\hat{y}_i^{(b)}=\sum_{k=0}^{b}{\hat{r}_i^{(k)}} = \hat{y}_i^{(b-1)}+\hat{r}_i^{(b)} \ et \ \hat{y}_i^{(0)}=\hat{h}(x_i), \ 1 \leq b \leq B, 1 \leq i \leq n\end{equation}

On définit également $\Omega$ une fonction qui prend en entrée un modèle (un arbre de décision par exemple) et renvoie une mesure de la complexité du modèle.
L'algorithme se présente comme ceci:
\begin{itemize}
    \item Initialisation: on définit un modèle constant $\hat{h_0}$. Par exemple: $\hat{h_0}(x_i)=C, 1 \leq i \leq n$, avec $C \in \mathds{R}$. Par exemple $C=0$.  On obtient $\hat{y}^{(0)}=\hat{r}^{(0)}=C$
    \item Pour b allant de 1 à B:
    \begin{itemize}
        \item Calibrage du modèle $M_b$ et de la fonction $\hat{h_b}$ associée, ajustés sur les données $(x,y-\hat{y}^{(b-1)})$ avec $y-\hat{y}^{(b-1)}=\hat{r}^{(b)}$. c'est-à-dire que $\hat{h}_b(x_i)$ donne une estimation de $y_i-\hat{y_i}^{(b-1)}, 1 \leq i \leq n$
        en optimisant la fonction de coût: \begin{align}
        \hat{h_b} &=\underset{h_b \in H}{argmin}\sum\limits_{i=1}^{n}{j(y_i,\hat{y_i}^{(b)})} + \sum\limits_{l=1}^{b}{\Omega(h_l)}\\&=\underset{h_b \in H}{argmin}\sum\limits_{i=1}^{n}{j(y_i,\hat{y_i}^{(b-1)}+h_b(x_i))} +\Omega(h_b) + C_b 
        \label{XGBoost}
        \end{align} 
        avec $C_b$ une constante qui dépend seulement des itérations avant b. Dans le cas d'une fonction de coût MSE, on obtient: 
        \begin{equation}
        \hat{h}_b=\underset{h_b \in H}{argmin}\sum\limits_{i=1}^{n}{(y_i-(\hat{y_i}^{(b-1)}+h_b(x_i))^2} +\Omega(h_b) + C_b \end{equation}
        Soit: \begin{equation} \hat{h}_b = \underset{h_b \in H}{argmin}\sum\limits_{i=1}^{n}{[2 (\hat{y_i}^{(b-1)}-y_i)h_b(x_i)+h_b(x_i)^2]} +\Omega(h_b) + C_b\end{equation}
        
        La forme obtenue, avec un terme d'ordre 1 et d'ordre 2, peut également être retrouvée dans le cas de fonctions de coût différentes de la MSE, en utilisant son développement de Taylor à l'ordre 2:\\
        \begin{equation}\hat{h}_b=\underset{h_b \in H}{argmin}\sum\limits_{i=1}^{n}{l(y_i,\hat{y_i}^{(b-1)})+ \alpha_i^{(b)} h_b(x_i)+\frac{1}{2}\beta_i^{(b)} h_b(x_i)^2} +\Omega(h_b) + C_b\end{equation}
        avec: \begin{itemize}
            \item $\alpha_i^{(b)} = \frac{\partial j}{\partial y}(y_i,\hat{y}^{(b-1)})$
            \item $\beta_i^{(b)} = \frac{\partial^2 j}{\partial y^2}(y_i,\hat{y}^{(b-1)})$
        \end{itemize}
        Il s'agit d'une approximation licite car les termes $h_b(x_i)$ sont supposés de taille négligeable étant donné qu'il s'agit de classifieurs faibles.\\
        Ainsi, en supprimant toutes les constantes (qui dépendent des étapes précédant l'étape b), on doit résoudre le problème d'optimisation suivant: 
        \begin{equation}\hat{h}_b=\underset{h_b \in H}{argmin}\sum\limits_{i=1}^{n}{\alpha_i^{(b)} h_b(x_i)+\frac{1}{2}\beta_i^{(b)} h_b(x_i)^2} +\Omega(h_b)\end{equation}
        C'est comme ceci que XGBoost fonctionne: il peut optimiser chaque fonction de perte choisie, en utilisant le même solveur en prenant les coefficients $\alpha_i^{(b)}$ et $\beta_i^{(b)}$ comme input.
       
    \end{itemize}
     \item Finalement, à la fin de notre algorithme, notre estimation de $y$ est donnée par $\hat{y}^{(B)}$: il s'agit de notre output.
\end{itemize}

\paragraph{Complexité du modèle et régularisation \\}
Nous avons présenté dans l'algorithme une fonction de complexité $\Omega$. Cette fonction contient un terme de régularisation afin d'éviter le surapprentissage. Plaçons nous dans le cas où les classifieurs faibles utilisés sont des arbres. Notons T le nombre de feuilles au dernier niveau de l'arbre, $w_t$ le score prédit par la feuille $t$ ( $1 \leq t \leq T$). La fonction $h_b$ associée à l'arbre de l'itération $b$ ($1 \leq b \leq B$) est définie par:
$h_b(x_i)=w_{s(x_i)}$, avec $s:\mathds{R}^p \rightarrow \{1,...,T\}$ une fonction renvoyant le numéro de la feuille associée au point considéré.
Avec une écriture vectorielle, on a: $h_b(x)=w_{s(x)}$.
La fonction de complexité du XGBoost est alors généralement définie par: \begin{equation}\Omega(h)=\gamma T + \frac{1}{2} \lambda \sum\limits_{k=1}^{T}{w_k^2}\end{equation} où $\gamma$ et $\lambda$ sont des paramètres de régularisation à choisir.

\paragraph{Algorithme de construction des arbres \\}
En reprenant, notre formule d'optimisation: $\sum\limits_{i=1}^{n}{\alpha_i^{(b)} h_b(x_i)+\frac{1}{2}\beta_i^{(b)} h_b(x_i)^2} +\Omega(h_b)$ et en injectant notre fonction de complexité définie juste avant, on obtient:
\begin{equation}\sum\limits_{i=1}^{n}{\alpha_i^{(b)} h_b(x_i)+\frac{1}{2}\beta_i^{(b)} h_b(x_i)^2} +\gamma T + \frac{1}{2} \lambda \sum\limits_{k=1}^{T}{w_k^2}\end{equation} \\
Soit, en intervertissant les sommes:
\begin{equation}\sum\limits_{j=1}^{T}{\begin{bmatrix}(\sum\limits_{i \in I_j}{\alpha_i^{(b)}})w_j+\frac{1}{2}(\sum\limits_{i \in I_j}{\beta_i^{(b)}}+\lambda)w_j^2\end{bmatrix}+\gamma T}\end{equation} 
avec $I_j=\{i \in \{1,...,T\} | s(x_i)=j\}$ l'ensemble contenant tous les indices des points qui ont été conduits à la feuille j.
En notant $A_j=\sum\limits_{i \in I_j}{\alpha_i^{(b)}}$ et $B_j=\sum\limits_{i \in I_j}{\beta_i^{(b)}}$, on obtient: 
\begin{equation}\sum\limits_{j=1}^{T}{[A_j w_j+\frac{1}{2}(B_j+\lambda)w_j^2]+\gamma T}\end{equation}
Dans cette équation les scores de prédiction $w_j$ n'interagissent pas entre-eux et sont donc indépendants. Pour une fonction $s(x)$ donnée, on peut optimiser chaque terme de la somme indépendamment, à savoir: $A_j w_j+\frac{1}{2}(B_j+\lambda)w_j^2$.\\
Finalement on obtient, en excluant la solution $w_j=0$:
\begin{equation} \forall j \in \{1,...,T\}, w_j=-\frac{A_j}{B_j+\lambda}\end{equation}
et une fonction objectif associée valant alors: $-\frac{1}{2} \sum\limits_{j=1}^{T}{\frac{A_j^2}{B_j+\lambda}}+\gamma T$, qui mesure à quel point l'arbre associé à la fonction $s$, est bon (en terme de prédiction et de complexité).
Il faut à présent trouver le meilleur arbre, avec la fonction de tri $s$ la plus performante associée. Il faudrait en théorie énumérer tous les arbres possibles et choisir le meilleur mais cela demanderait trop de temps. 
Une méthode utilisée en pratique est une optimisation étage par étage de l'arbre. L'idée est de regarder si l'ajout de nouvelles feuilles à un niveau donné fournit un gain comparé à l'arbre initial, tout en tenant compte de la régularisation. Dans le cas de l'ajout de deux feuilles à un niveau donné, il faut que le gain associé (régularisé) soit positif :
\begin{equation}Gain=\frac{1}{2}\begin{bmatrix}\frac{A_G^2}{B_G+\lambda}+\frac{A_L^2}{B_L+\lambda}-\frac{(A_G+A_L)^2}{B_G+B_L+\lambda}\end{bmatrix}-\gamma\end{equation}
L'indice G réfère à la feuille gauche ajoutée, et D à la feuille droite.
Finalement il faut que le gain d'ajout de ces deux feuilles, comparé à la situation précédente, soit supérieur au coefficient $\gamma$ de régularisation. 
Ainsi, pour construire un arbre, on cherche récursivement la meilleure division possible jusqu'à ce qu'on atteigne la profondeur maximale.
Ensuite, on élague les noeuds avec un gain négatif avec une approche du bas vers le haut (bottom-up).

\subsubsection{Avantages du XGBoost}
Les avantages de l'algorithme XGBoost sont nombreux, et peuvent expliquer pourquoi il est tant utilisé dans les compétitions de Machine Learning.
\begin{itemize}
    \item Il existe de nombreux hyperparamètres que l'on peut régler au plus fin pour optimiser ses performances. Ils permettent de garder un contrôle sur le compromis biais/variance. On peut citer notamment:
    \begin{itemize}
    \item[$\bullet$] Paramètres de contrôle de la complexité du modèle :
    \begin{itemize}
      \item[$\cdot$] Le nombre de sous-arbres $h_m$ entraînés 
     \item[$\cdot$] La profondeur maximale de chaque arbre $h_m$
     \item[$\cdot$] Gain minimum $\gamma $ requis pour autoriser une division supplémentaire
    \end{itemize}
    \item[$\bullet$] Paramètres de robustesse au bruit :
    \begin{itemize}
        \item[$\cdot$] Ratio de sous échantillonnage de la base d'apprentissage, compris entre 0 et 1
        \item[$\cdot$] Ratio de sous-échantillonnage des colonnes lors de la construction de chaque arbre 
    \end{itemize}
    \item[$\bullet$] Le taux d'apprentissage (\emph{learning rate}). Il s'agit du coefficient utilisé dans la méthode de descente du gradient pour contrôler la vitesse de convergence de l'algorithme. Si il est trop bas, le temps de convergence peut être long, et si il est trop élevé, l'algorithme risque de ne pas converger.
    \item[$\bullet$] Les paramètres $\gamma$ et $\lambda$  de régularisation $\mathds{L}^1$ et $\mathds{L}^2$.
    \item[$\bullet$] Ajustement possible dans le cas d'une classification avec des données déséquilibrées entre les classes (en utilisant par exemple la métrique "AUC").
\end{itemize}
    \item Rapidité de calcul, en comparaison du Tree Gradient Boosting classique.
\end{itemize}
