# Supplementary material for: Applying Machine Learning to Life Insurance: some knowledge sharing to master it
Source: arXiv:2209.02057 source file (2022-09-27)
Supplement: Supplementary file 3 [file appendix.tex]

\chapter{About the data (Antoine)}

\section{Analysis and frame}

The SEER database contains 1,548,199 records breast cancers diagnosed from 1973 to 2014. The data base is composed of 4 directories covering different registries and period of observation.

Certain patient are diagnosed for a breast cancer more than once. The inclusion of "duplicated" data is not considered relevant for the study. Here, the first record is only considered.

Over the years, the definition of the variable and the quality of the measurement changed. The period of observation is from 01/01/2004 to 31/12/2014. A consistent set of variable is defined with no changes over these 11 years.

Certain missing data must be removed from the data set. In the period of study, 33 patients are not recorded with an age at diagnosis and 2,809 patients have an unknown survival time. This represents less than 0.4\% of the data set.

The event is defined as a death of a cancerous patient from the breast cancer. In fact, many insured are diagnosed with a breast cancer but their death is caused by another health issue. In order to study the over mortality due to the breast cancer, only the deaths caused by the breast cancer are positive event. All other deaths caused by another cancer or non cancer sites are right-censored.

At the diagnosis, the stage of the cancer is assessed according to several features (size of tumor, extension, lymph nodes, ...). A breast cancer is a Carcinomas in Situ (CiS) when the tumour is confined to its original location and has not invaded the surrounding organs/tissues. Once the tumour is removed by a surgical practitioner, the patient is very likely to cure. The other stages have a worst prognosis. CiS are usually not covered by CI policies. All data recorded with a CiS behaviour are removed of the data set.

%Include survival curves per staging

In a nutshell, the database only includes 592,694 non duplicated data of patient suffering of a breast cancer. CiS, missing age at diagnosis and missing survival times are not included in the study.

\section{Partition}

The comparison of the models is possible if each model is trained on the same partition of the data. In this study, we have decided to split the data set into 5 folds of 90,000 data and one hold out that contains the remaining observations. All data are uniformly shuffled before the partitioning.

% Insert global mortality for each folds and population per fold

\section{Features list and description}

The data set contains 86 non-empty variables. A large number of variable are excluded of the analysis since their quality is too low or the information is duplicated in another variable.

Some variable encode the same information but with different coding rules : new staging definition, re-code of a detailed variable, ... The homogeneous sets of variables have been gathered in the table ??.

\begin{center}
\begin{tabular}{|r|l|l|l|}\hline
Description & Variables & Selected & Missing/unknown code \\ \hline\hline
Race & RACE RAC\_RECA RAC\_RECY & RAC\_RECY & 9\\
Hispanic & NHIA NHIAREC & NHIAREC & \\
Gender & SEX & SEX & \\
Age at diagnosis & AGE\_DX & AGE\_DX & \\
Primary site & SITEO2V & SITEO2V & \\
Laterality & LATERAL & LATERAL & 9 \\
Histology & ICDOT10V, ICDOT9V, HIST\_REC & SITEO2V (primary site) & \\
Grading & GRADE & GRADE & 9\\
Number of positive nodes & EOD10\_PN CS\_SSF3 & EOD10\_PN & 95 97 98 99\\
Number of nodes explored & EOD10\_NE & EOD10\_NE & 95 96 97 98 99\\
Size of tumour & CS\_SIZE & CS\_SIZE (+ creation MICRO\_FOCI) & 996 997 998 999\\
Lymphatic nodes & CS\_NODE & CS\_NODE & 999\\
Extension & CS\_EXT & CS\_EXT & 999 950\\
Metastasis & CS\_METS & CS\_METS & 99\\
Estrogen receptor & ERSTATUS CS\_SSF1 & ERSTATUS & 4\\
Progesterone receptor & PRSTATUS CS\_SSF2 & PRSTATUS & 4\\
Immunochemistry (IHC) & CS\_SSF4 & CS\_SSF4 & 987\\
Molecular (MOL) studies of regional nodes & CS\_SSF5 & CS\_SSF5 & 987\\
Size of tumour invasive components & CS\_SSF6 & CS\_SSF6 & 987\\
AJCC tumour size & D\_AJCC\_T ADJTM\_6VALUE & D\_AJCC\_T & 88 99\\
AJCC node & D\_AJCC\_N ADJNM\_6VALUE & D\_AJCC\_N & 88 99\\
AJCC metastasis & D\_AJCC\_M ADJM\_6VALUE & D\_AJCC\_M & 88 99\\
AJCC stage & D\_AJCC\_S ADJAJCCCSTG & D\_AJCC\_S & 88 99\\
Summary SEER staging & D\_SSG77 D\_SSG00 HST\_STGA HIST\_SSG\_2000 & D\_SSG00 & 9\\
Primary surgery & SURGPRIM & SURGPRIM & 90 99\\
Other surgery & SURGOTH & SURGOTH & 9\\
Reason for no surgery & NO\_SURG & NO\_SURG & 9 8\\
First primary tumour & FIRSTPRM & FIRSTPRM & \\
Site/Histology child adolescent & ICCC3WHO ICCC3XWHO AYA\_RECODE & ICCC3WHO & 999\\
Evaluation CS extension/size & EXTEVAL & EXTEVAL & 9\\
Evaluation node & NODEEVAL & NODEEVAL & 9\\
Evaluation metastasis & METSEVAL & METSEVAL & 9\\
Human Epidermal Growth Factor Receptor 2 & HER2 CS\_SSF15 & HER2 & 9\\ \hline
\end{tabular}
\end{center}

\section{Survival statistics}

\subsection{Race}

The ethnicity of the patient is a key risk factor. Black people have a higher mortality than the whites and Asian have a better prognosis after the diagnosis. 

\begin{center}
\includegraphics[scale=0.4]{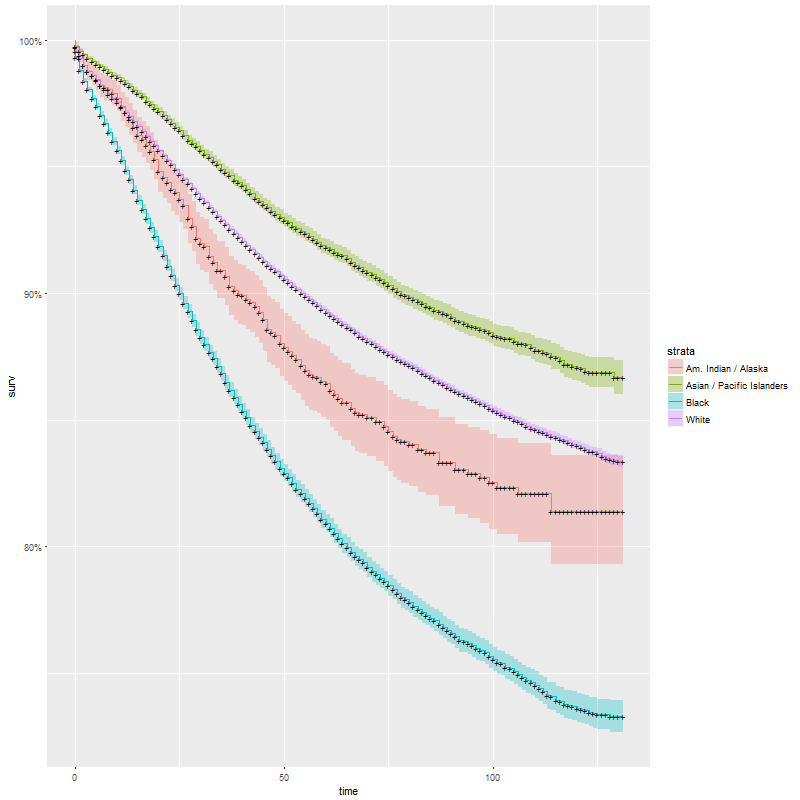}
\captionof{figure}{Survival plot per race}
\label{figure_statsdesc_race}
\end{center}

\subsection{Hispanic}

\begin{center}
\includegraphics[scale=0.4]{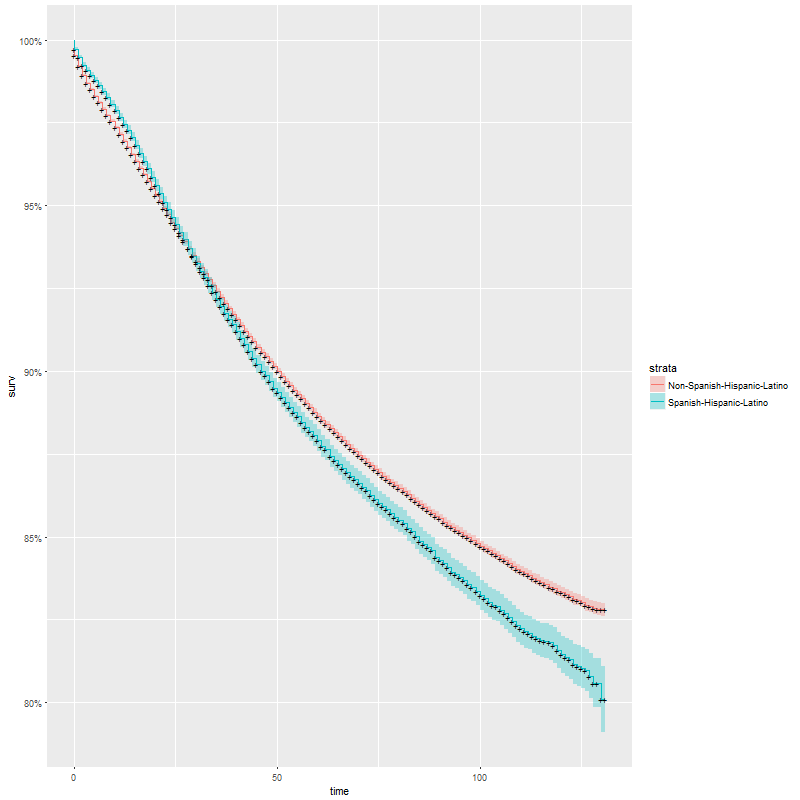}
\captionof{figure}{Survival plot per hispanic}
\label{figure_statsdesc_nhiarec}
\end{center}

\subsection{Gender}

The data set contains 4809 men and 587,825 females. As depicted on the figure \ref{figure_statsdesc_sex}, the breast cancer for males is frequently less curable than the breast cancer for females.

\begin{center}
\includegraphics[scale=0.4]{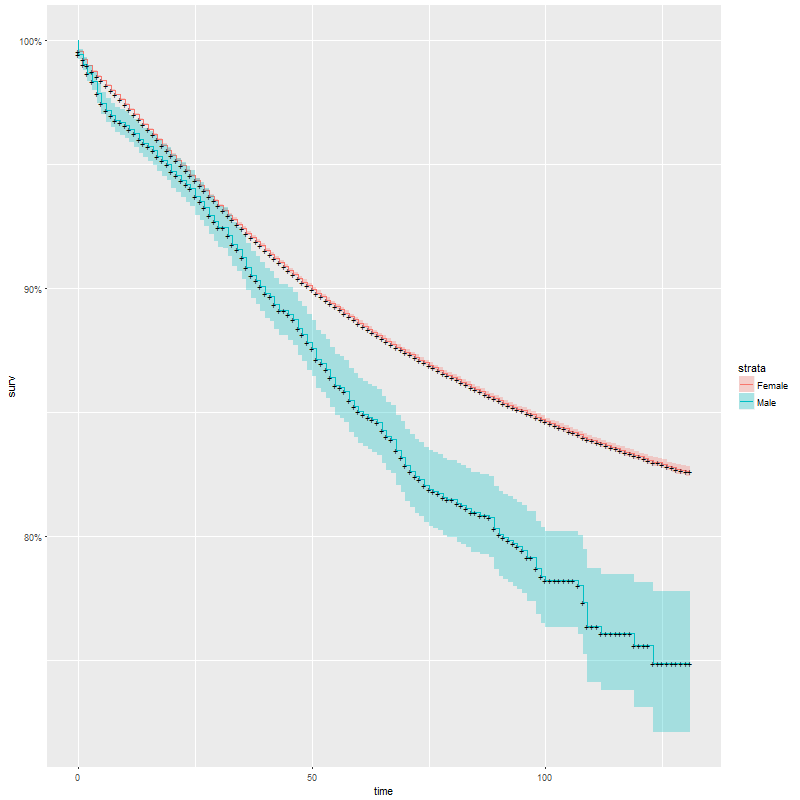}
\captionof{figure}{Survival plot per gender}
\label{figure_statsdesc_sex}
\end{center}

\subsection{Age at diagnosis}

The 4 classes of the continuous variable Age at diagnosis have been calibrated with a decision tree of max depth 3.

\begin{center}
\includegraphics[scale=0.4]{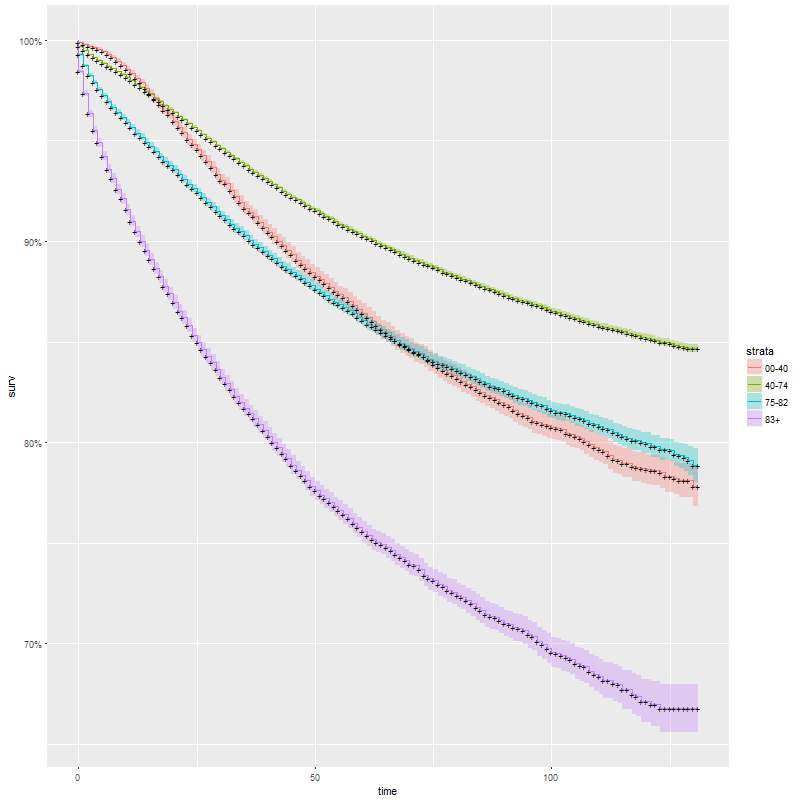}
\captionof{figure}{Survival curves per age band}
\label{figure_statsdesc_age}
\end{center}

\subsection{Positive node number}

The number of positive regional nodes is highly correlated with the advancement of the illness. The presence of metastasis in the nodes surrounding the tumor is a very bad sign for the patient. The medical expert frequently remove the invaded nodes but metastasis can have spread farther the explored location.  

\begin{center}
\includegraphics[scale=0.4]{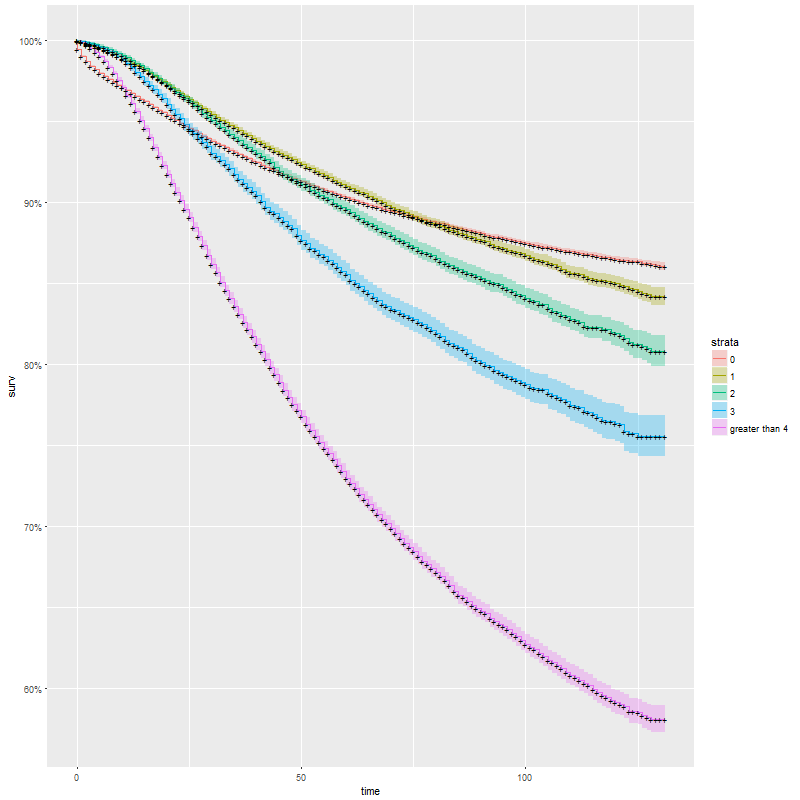}
\captionof{figure}{Survival curves per positive node bands}
\label{figure_statsdesc_positiveNode}
\end{center}

\subsection{Explored nodes}

\begin{center}
\includegraphics[scale=0.4]{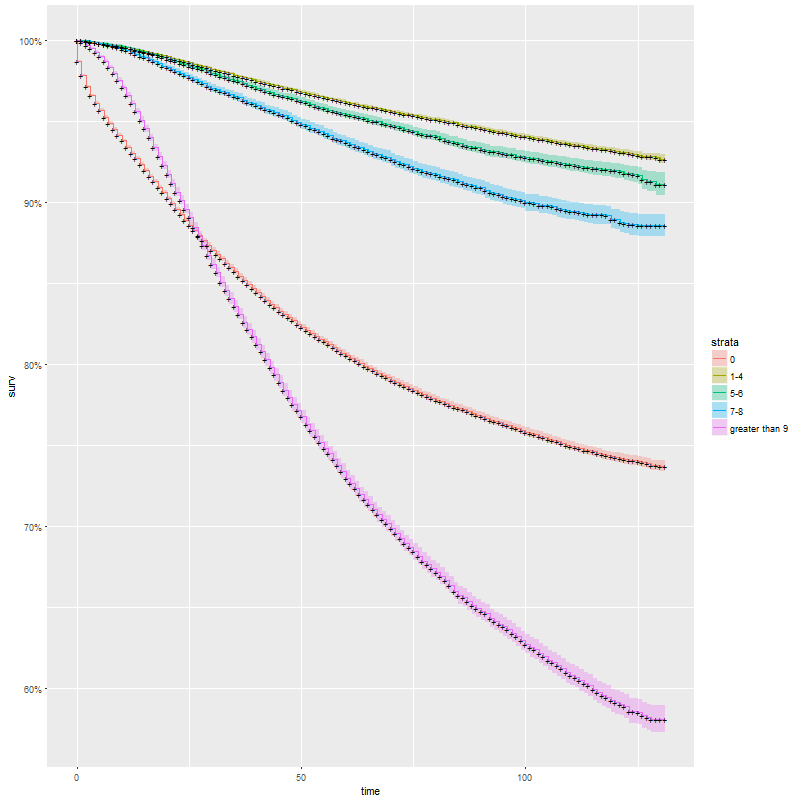}
\captionof{figure}{Survival curves per explored node bands}
\label{figure_statsdesc_exploredNode}
\end{center}

\subsection{Tumor size}

The size of the tumor is a key risk factor for the patient. The bigger the tumor, the more likely the cancerous cells can infect other tissues or organs. The figure \ref{figure_statsdesc_size} represents the five survival curves associated to the five most relevant bands of tumor size. The boundaries intervals have been calibrated with a survival tree.

\begin{center}
\includegraphics[scale=0.4]{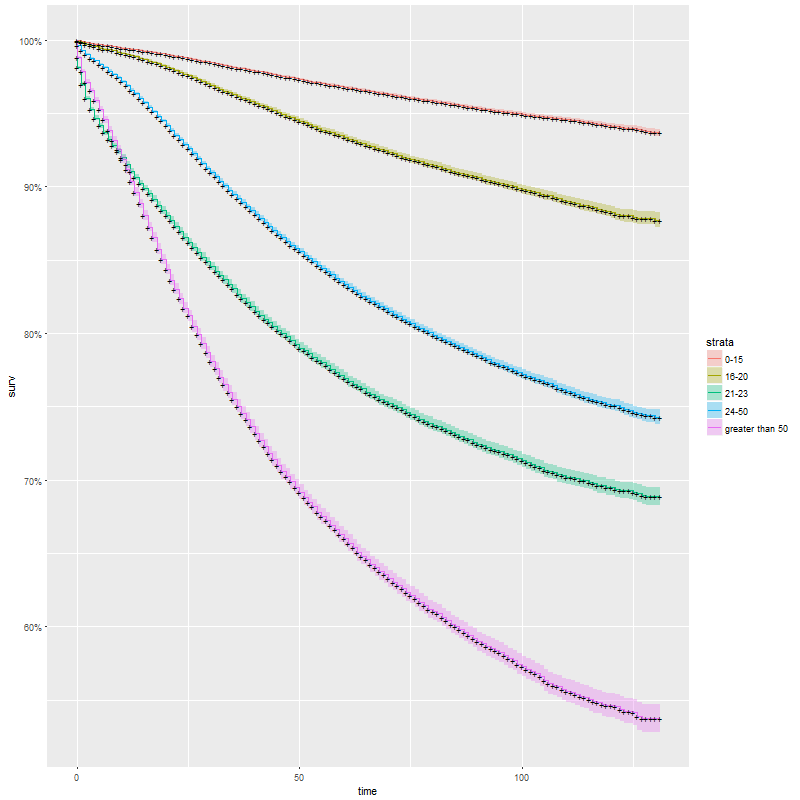}
\captionof{figure}{Survival curves per tumour size bands}
\label{figure_statsdesc_size}
\end{center}

\subsection{Grade}

\begin{center}
\includegraphics[scale=0.4]{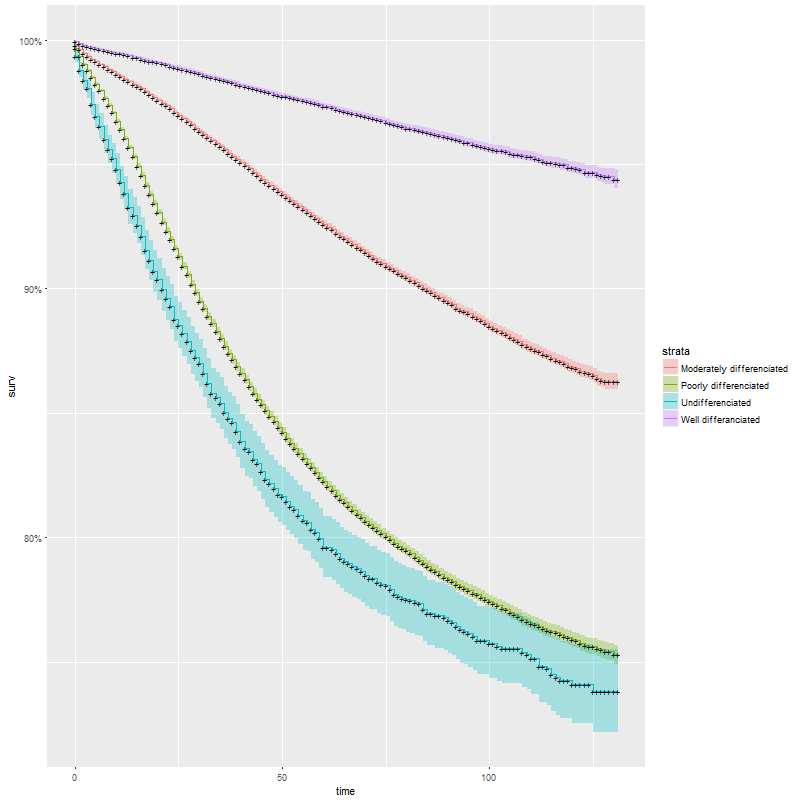}
\captionof{figure}{Survival curves per grade}
\label{figure_statsdesc_grade}
\end{center}

\subsection{Stage}

The AJCC staging is a classification of a cancer according to four main factors:
\begin{itemize}
    \item cancer site
    \item size of the primary tumor
    \item lymphatic nodes involvement
    \item presence of metastasis
\end{itemize}

The severity of the patient's cancer is ranked. The prognosis of the patient deteriorates when the stage grows. The figure \ref{figure_statsdesc_race} contrasts the poores / best stages and survival curves.

\begin{center}
\includegraphics[scale=0.4]{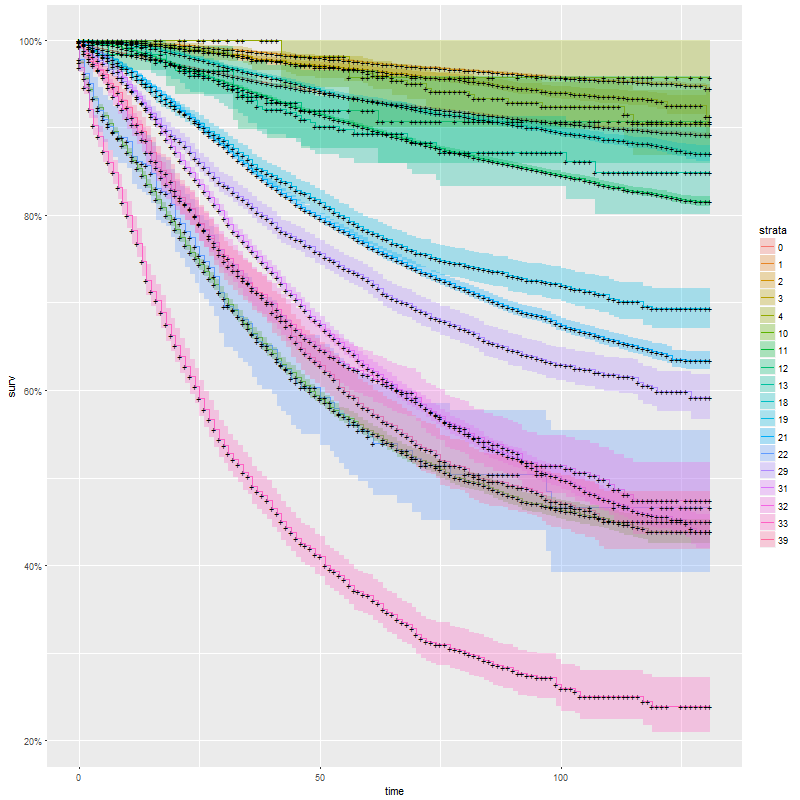}
\captionof{figure}{Survival curves per stage}
\label{figure_statsdesc_D_AJCC_S}
\end{center}

\chapter{Notations and Definitions}

\chapter{Survival modelling}

\chapter{Additional results}

\chapter{Other}
