# Supplementary material for: Applying Machine Learning to Life Insurance: some knowledge sharing to master it
Source: arXiv:2209.02057 source file (2022-09-27)
Supplement: Supplementary file 4 [file log_xgboost.tex]

\chapter{Logistic regression for censored data}
\\
At age x, the calculation of the exposures under the Balducci assumption lead to the following conclusions:
\begin{itemize}
  \item If the patient survive the perid or exit the study, the exposure $E_{ix}$ will be the period of observation of the individual
  \item If the patient dies between age and age+1, the exposure $E_{ix}$ is set to 1
\end{itemize}

Under this assumption, the mortality rate for cohort age is $q_x = \frac{d_x}{E_x}$.

To estimate $q_x$, let's assume that the death event is a bernoulli variable $B(\mu)$.

The likelihood becomes:
$L(q_x) = \prod_{i=1}^{n} q_x^{d_i}(1-q_x)^{1-d_i}$

The log likelihood is:
$l(q_x) = \sum_{i=1}^{n} d_i log(q_x) + (1-d_i)log(1-q_x)$

Solving $\frac{d l(q_x)}{d q_x} = 0$, we show that this estimator converge toward $\hat{q_x} = D/n$ which is incorrect (with $D = \sum_{i=1}^{n} d_i$).

If we plugin the balducci exposure as weights in the log likelihood $E_{ix}$, we get the modified log likelihood as follow:
$l(q_x) = \sum_{i=1}^{n} E_{ix} d_i log(q_x) + E_{ix} (1-d_i)log(1-q_x)$

The derivative is
$\frac{d l(q_x)}{d q_x} = \sum_{i=1}^{n} E_{ix} \frac{d_i}{q_x} - E_{ix} \frac{1-d_i}{1-q_x}$

Thus,
$\frac{\sum_{i=1}^{n}E_{ix}d_i}{\hat{q_x}} = \frac{\sum_{i=1}^{n}E_{ix}-\sum_{i=1}^{n}E_{ix}d_i}{1-\hat{q_x}}$

And
$\hat{q_x} = \frac{\sum_{i=1}^{n}E_{ix}d_i}{\sum_{i=1}^{n}E_{ix}}$

Under the balducci assumption, $E_{ix}$ are equal to 1 for the dead. The previous expression can be simplified:
$\hat{q_x} = \frac{\sum_{i=1}^{n}d_i}{\sum_{i=1}^{n}E_{ix}}$.

To conclude, it seems that the injection of the Balducci exposure in the log likelihood allow to take into account the partial information due to the presence of censorship.

The log likelihood can be simplified:\\
$l(q_x) = \sum_{i=1}^{n} E_{ix} + \sum_{i=1}^{n} E_{ix} d_i log(\frac{q_x}{1-q_x})$

\chapter{Mortality XGBoost}
Using the original notation of the xgboost paper, https://arxiv.org/pdf/1603.02754.pdf.

At time t, we have:
\begin{equation}
    L^{(t)} = \sum_{i=1}^{n} l(y_i, \hat{y_i}^{(t-1)} + f_t(x_i)) + \Omega(f_t) \approx \sum_{i=1}^{n} l(y_i, \hat{y_i}^{(t-1)}) + g_i f_t(x_i) + \frac{1}{2} h_i f_t(x_i)^2 + \Omega(f_t)
\end{equation}

In our case, we are interested at examining the gradient boosting for:
\begin{equation}
    l(y_i, \hat{y_i}^{(t-1)} + f_t(x_i)) = ec_i y_i log(\frac{1}{1+e^{\hat{y_i}^{(t-1)} + f_t(x_i)}}) + ec_i (1-y_i) log(1-\frac{1}{1+e^{\hat{y_i}^{(t-1)} + f_t(x_i)}})
\end{equation}

The gradient
\begin{equation}
    g_i = ec_i y_i - ec_i \frac{1}{1+e^{\hat{y_i}^{(t-1)}}} = ec_i y_i - ec_i \hat{q_x}^{(t-1)}(x_i)
\end{equation}
With a loss function, the log likelihood we see that the gradient for each instance $i$ is proportional to the difference between the observed deads and the predicted  deads weighted by the central exposure. More importance is given to the observations with a bad mortality predictions.

The hessian
\begin{equation}
    h_i = - ec_i \frac{e^{\hat{y_i}^{(t-1)}}}{(1+e^{\hat{y_i}^{(t-1)})^2}} =  - ec_i \hat{q_x}^{(t-1)}(x_i) (1 - \hat{q_x}^{(t-1)}(x_i))
\end{equation}

The optimal weight
\begin{equation}
    w_j^* = - \frac{\sum_{i \in I_j} ec_i y_i - ec_i \hat{q_x}^{(t-1)}(x_i)}{- \sum_{i \in I_j} ec_i \hat{q_x}^{(t-1)}(x_i) (1 - \hat{q_x}^{(t-1)}(x_i)) + \lambda}
\end{equation}

The value of the weight $w_j^*$ can be high and the initial second order Taylor approximation is not sustainable. A shrinkage factor $\eta$ can be here introduce to diminish the importance of the current learner.\\

[Antoine C] Should I speak about the hessian being diagonal guaranteeing the decroissance of the loss function at each step (even a small one).

The scoring function for the weak learner t is
\begin{equation}
    L^t(q) = - \frac{1}{2} \sum_{j=1}^T  \frac{\sum_{i \in I_j} ec_i y_i - ec_i \hat{q_x}^{(t-1)}(x_i)}{- \sum_{i \in I_j} ec_i \hat{q_x}^{(t-1)}(x_i) (1 - \hat{q_x}^{(t-1)}(x_i)) + \lambda} + \gamma T
\end{equation}

The litterature also recommends to use some subsampling when constructing the tree to diminish the greediness of the trees.\\

In a word, the xgboost corrected with the central exposure is a model that will correctly integrate the partial information for each duration where an individual is observed. The learners recursively segment the space with weights dependant on the performance of the precedent learners and the regularisation parameters. This dependency leads to difficulties in the analysis of the structure of the trees. However, the celebrity of the xgboost is done and the model has demonstrated high performances in many data science competition.
